# Supplementary material for: Accurate Determination of the Neutron Skin Thickness of $^{208}$Pb through Parity-Violation in Electron Scattering
Source: arXiv:2102.10767 ancillary file (2021-04-27)
Supplement: Supplementary file 1 [file Supplemental_Material.pdf]

# Supplementary Material

(The PREX Collaboration)

## MODEL UNCERTAINTY IN $R_W$

To quantify the model uncertainty we fit theoretical weak charge densities  $\rho_W(r)$  from a large variety of non-relativistic and relativistic density functional models to a two-parameter Fermi function  $\rho_W(r, c, a)$  [1, 2]

$$\rho_W(r, c, a) = \rho_W^0 \frac{\sinh(c/a)}{\cosh(r/a) + \cosh(c/a)}. \quad (1)$$

Here, the parameter  $c$  describes the size of the nucleus while  $a$  describes the surface thickness. The interior weak density  $\rho_W^0 = 3Q_W/[4\pi c(c^2 + \pi^2 a^2)]$ , with  $Q_W$  being the weak charge of a nucleus. The fits suggest the range of uncertainty  $a = 0.605 \pm 0.025$  fm (see Table I), reflected in the model uncertainty lines (dashed red) in Fig. 3 of the main text. See further details in [3].

| Model        | $a[{}^{208}\text{Pb}]$ (fm) |
|--------------|-----------------------------|
| Big Apple[4] | 0.6087                      |
| FSUgold [5]  | 0.6134                      |
| IUFSU [6]    | 0.6079                      |
| NL3[7]       | 0.6096                      |
| SIH [8]      | 0.5792                      |
| SLY4 [9]     | 0.6040                      |
| TAMUc [10]   | 0.6351                      |
| TAMUb [10]   | 0.6210                      |
| TAMUa [10]   | 0.6125                      |

TABLE I. Surface thickness parameter  $a$  of Fermi function fits to the weak charge densities of  ${}^{208}\text{Pb}$ , see Eq. 1.

## ACCEPTANCE FUNCTION

The acceptance function  $\epsilon(\theta)$  describes the relative acceptance as a function of the lab-frame polar scattering angle. The function is generated through Monte Carlo simulation to match the observed distributions of the scattered momentum and angle. The simulation takes into account the geometric acceptance and spectrometer magnetic fields, as well as the initial and final state radiation, energy loss, and multiple scattering within the target. An uncertainty is ascribed to the acceptance function, which corresponds to the maximum variation in calculated  $\langle A_{PV} \rangle$  (using the FSUgold nuclear model [6]) for a family of simulation models that describe possible variations in the experimental acceptance while still reproducing the observed average scattering angle  $\langle \theta_{\text{lab}} \rangle$  or 4-momentum transfer squared  $\langle Q^2 \rangle$ .

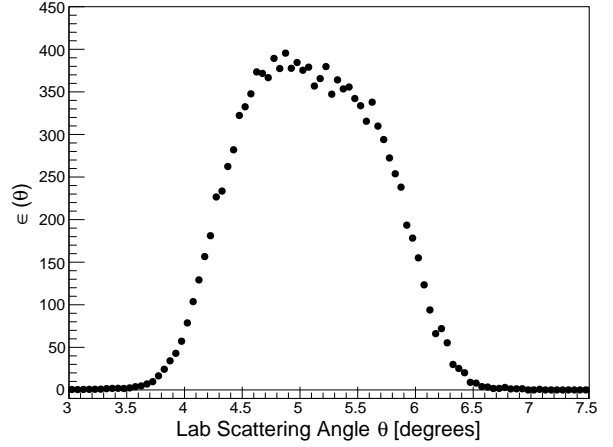

FIG. 1. Acceptance function  $\epsilon(\theta)$  for the PREX-2 measurement.

Figure 1 shows the function  $\epsilon(\theta)$ , which is provided in 100 bins, from  $3^\circ$  to  $8^\circ$ . The provided function is arbitrarily normalized to sum to unity over the full acceptance:

$$\sum_i \epsilon(\theta_i) \sin(\theta_i) \Delta\theta = 1 \quad (2)$$

with  $\Delta\theta = 0.05^\circ$ .

- [1] D. W. L. Sprung and J. Martorell, The symmetrized fermi function and its transforms, J. Phys. A **30**, 6525 (1997).
- [2] J. Piekarewicz, A. R. Linero, P. Giuliani, and E. Chicken, Power of two: Assessing the impact of a second measurement of the weak-charge form factor of  ${}^{208}\text{Pb}$ , Phys. Rev. C **94**, 034316 (2016), arXiv:1604.07799 [nucl-th].
- [3] C. Horowitz, J. Piekarewicz, and B. Reed, Insights into nuclear saturation density from parity violating electron scattering, Phys. Rev. C **102**, 044321 (2020), arXiv:2007.07117 [nucl-th].
- [4] F. Fattoyev, C. Horowitz, J. Piekarewicz, and B. Reed, GW190814: Impact of a 2.6 solar mass neutron star on nucleonic equations of state, Phys. Rev. C **102**, 065805 (2020), arXiv:2007.03799 [nucl-th].
- [5] B. G. Todd-Rutel and J. Piekarewicz, Neutron-Rich Nuclei and Neutron Stars: A New Accurately Calibrated Interaction for the Study of Neutron-Rich Matter, Phys. Rev. Lett. **95**, 122501 (2005), arXiv:nucl-th/0504034.
- [6] F. Fattoyev, C. Horowitz, J. Piekarewicz, and G. Shen, Relativistic effective interaction for nuclei, giant resonances, and neutron stars, Phys. Rev. C **82**, 055803 (2010), arXiv:1008.3030 [nucl-th].
- [7] G. A. Lalazissis, J. Konig, and P. Ring, A new

- parametrization for the Lagrangian density of relativistic mean field theory, *Phys. Rev. C* **55**, 540 (1997), arXiv:nucl-th/9607039.
- [8] M. Beiner, H. Flocard, N. van Giai, and P. Quentin, Nuclear ground state properties and self-consistent calculations with the Skyrme interactions: 1. Spherical description, *Nucl. Phys. A* **238**, 29 (1975).
- [9] E. Chabanat, P. Bonche, P. Haensel, J. Meyer, and R. Schaeffer, A Skyrme parametrization from subnuclear to neutron star densities. 2. Nuclei far from stabilities, *Nucl. Phys. A* **635**, 231 (1998), [Erratum: *Nucl.Phys.A* 643, 441–441 (1998)].
- [10] F. J. Fattoyev and J. Piekarewicz, Has a thick neutron skin in  $^{208}\text{Pb}$  been ruled out?, *Phys. Rev. Lett.* **111**, 162501 (2013), arXiv:1306.6034 [nucl-th].
